# Supplementary material for: Comprehensive Molecular-level Understanding of MgO Hydration through Computational Chemistry
Source: arXiv:2601.10186 ancillary file (2026-01-15)
Supplement: Supplementary file 1 [file manuscript_SI.pdf]

# Supporting Information for:

# Comprehensive Molecular-level Understanding of MgO Hydration through Computational Chemistry

Taichi Inagaki*,† and Miho Hatanaka†,‡

*Department of Chemistry, Faculty of Science and Technology, Keio University, 3-14-1 Hiyoshi, Kanagawa 223-8522, Japan, and Institute for Molecular Science, Okazaki, Aichi 444-8585, Japan*

E-mail: taichi.inagaki@keio.jp

*To whom correspondence should be addressed

†Department of Chemistry, Faculty of Science and Technology, Keio University, 3-14-1 Hiyoshi, Kanagawa 223-8522, Japan

‡Institute for Molecular Science, Okazaki, Aichi 444-8585, Japan

**Contents**:


1. Computational Methods
   1.1. PS-MD simulations for structure generation
   1.2. DFTB and DFT calculations for structure refinement
   1.3. Simulation system and conditions
   1.4. NEB calculations for $Mg^{2+}$ dissolution
   1.5. PS-MD simulations for nucleation in water
2. Potential Energy Variation of Interfacial Structures
3. Supplementary Tables and Figures

# 1 Computational Methods

## 1.1 PS-MD simulations for structure generation

Generally, there are two common approaches for theoretically investigating solid-state chemical reactions. The first approach involves assuming elementary processes, defined by reaction coordinates, and changing the interfacial molecular structures along these coordinates using static first-principles calculations. This method can identify the product structures of these elementary processes and estimate the associated energy changes. Furthermore, it can sometimes provide insights into the reaction kinetics by locating transition states and determining their reaction barrier heights. For heterogeneous and complex solid surfaces, however, it is often difficult to presuppose appropriate reaction coordinates. The second approach is to observe interfacial structural changes using molecular dynamics (MD) simulations. The appeal of this method lies in its ability to capture the reaction processes and their correct dynamics without the need to assume reaction coordinates. Nevertheless, due to the limited timescales accessible to conventional MD simulations, this method can typically handle only chemical reactions with very low energy barriers, which often results in minimal structural changes.

In this study, we employed an approach for generating a series of stable structures associated with chemical reactions of interest without assuming any elementary processes. The structure generation method is based on MD simulations but introduces a potential scaling (PS) technique to enable chemical reactions.[S1] At each MD step, the potential energy surface (PES), $U(t)$, is continuously multiplied by a scaling factor $\alpha$ ($0 < \alpha < 1$), such that $U(t+dt) = \alpha U(t)$. This flattening of the PES lowers the reaction barriers and facilitates bond rearrangements and atomic migrations. This flattening process is carried out for a predetermined number of steps, $N_{\mathrm{PS}}/2$. Subsequently, the original PES is restored by reversing the scaling (i.e., dividing by $\alpha$) for the same number of steps ($N_{\mathrm{PS}}/2$), such that $U(t+dt) = U(t)/\alpha$. This restoration process allows the structure to relax into a new locally stable state. This entire procedure of flattening and restoration, spanning $N_{\mathrm{PS}}$ total steps, constitutes one PS-MD cycle. By repeating these PS-MD cycles,

we can induce significant interfacial structural changes. This scaling operation does not alter the relative potential energy landscape between different configurations. Consequently, the trajectory tends to follow regions where the original potential energy is low, leading to the automatic selection of elementary processes with low energy barriers. While previous MD simulation methods have utilized statically scaled PES for efficient conformational sampling,[S2–S4] our PS-MD method employs a dynamic scaling procedure. This dynamic procedure is expected to trace overall chemical reaction from the reactant state (MgO + $H_2O$) to the product state ($Mg(OH)_2$). Note that this dynamic scaling procedure does not follow Hamiltonian dynamics, which assumes a single, time-independent PES. This often injects additional energy into the system as kinetic energy and can lead to significant overheating.[S1] Therefore, in the present simulations, we employed a Langevin thermostat to prevent an extreme increase in kinetic energy. Furthermore, to ensure that the system is well-stabilized, relaxation MD simulations using the same thermostat were performed after each PS-MD cycle.

The computational details for the PS-MD simulations are as follows. One PS-MD cycle consisted of a total of 40,000 steps, comprising 10,000 steps of potential flattening, 10,000 steps of potential restoration, and 20,000 steps of relaxation MD without potential scaling. Here, $N_{\mathrm{PS}}$ was defined as 20,000, representing the combined number of steps for the potential flattening and restoration phases. A total of 1,000 PS-MD cycles were performed for each independent run. The scaling parameter $\alpha$ was set to 0.999, which results in a maximum scaling factor of approximately $4.5 \times 10^{-5}$ ($0.999^{N_{\mathrm{PS}}/2}$) applied to the potential energy (or the forces practically). This value of $\alpha$ was determined from preliminary test calculations based on achieving a balance between the simulation stability of integrating the equations of motion and the efficiency of key reactive events such as $Mg^{2+}$ dissolution and proton penetration. For example, using $\alpha$ = 0.9991, the dissolution of $Mg^{2+}$ ions was observed to be approximately an order of magnitude slower in terms of the number of PS-MD cycles required. This choice was made after other parameters (e.g., the number of MD steps, the MD timestep, and the damping parameter for the Langevin thermostat described below) were determined based on computational cost. The potential scaling was applied to all

atoms except for those in the bottom two layers of the MgO slab.

To allow for chemical bond rearrangements, the ReaxFF reactive force field[S5] was employed. The parameters in this study were based on those used by Zhu and co-workers,[S6] with some modifications, because the original parameters were not specifically tuned for the Mg-O-H system. Our modifications were primarily aimed at reproducing the correct orientation of water molecules on the MgO surface. Figure S1 illustrates the effect of the modifications by comparing the orientation of an adsorbed water molecule as obtained with the original parameters, our modified parameters, and a DFT calculation used as a reference. The modified reactive force field reasonably reproduces the slight H-down orientation observed in the DFT calculation. Further validation calculations demonstrate that the modified force field provides good qualitative accuracy (see Table S1). These validation results make our force field a significantly more reliable choice than another available force field[S7] that fails even to maintain the rock-salt structure of MgO. The force field file is provided as a supplemental material.

All PS-MD simulations were performed with a timestep of 0.5 fs using the LAMMPS program package,[S8] into which the PS scheme[S1] was implemented. The Langevin thermostat was used to maintain the system temperature at 300 K, with a damping parameter of 10 fs to ensure rapid dissipation. It should be noted that shorter damping times than 10 fs was found to hinder barrier crossings due to excessive random forces. The atoms in the bottom two MgO layers were constrained to their bulk crystal positions using harmonic tethering potentials with a force constant of 10.0 kcal/mol/Å$^2$. In this work, five independent PS-MD simulations were performed. Finally, it is crucial to note that in control simulations performed using a conventional *NVT* ensemble with the Langevin thermostat (i.e., without potential scaling), no chemical bond rearrangements, such as the breaking of Mg-O bonds in the solid surface, were observed.

(a) (b) (c)

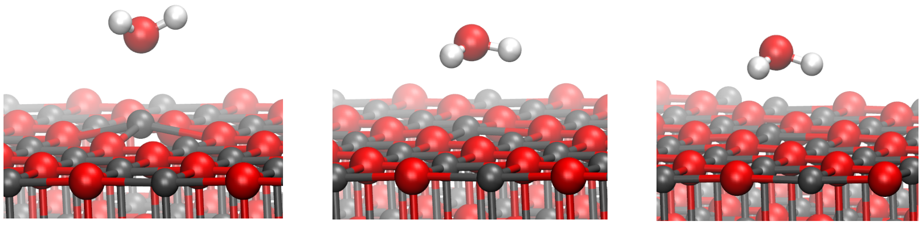

Figure S1: Orientation of a water molecule adsorbed on the MgO surface calculated using the original ReaxFF parameters (a), the modified ReaxFF parameters (b), and the DFT method (c). The details of the DFT calculation are given in Section 1.2 in Supporting Information.

Table S1: Comparison of Structural and Energetic Properties for the Mg-O-H System Calculated Using the ReaxFF, DFTB, and DFT Methods.[a]

| | ReaxFF | DFTB | DFT | Literature |
|---|---|---|---|---|
| MgO lattice constant | 4.280 | 4.313 | 4.156 | 4.211[c] |
| $Mg(OH)_2$ lattice parameters ($a$, $c$) | 3.081, 4.765 | 3.170, 4.369 | 3.136, 4.542 | 3.142, 4.766[d] |
| Reaction energy | −37.7(−35.5) | −24.1(−23.9) | −23.5(−19.0) | −19.5[e] |
| MgO surface energy | 0.78 (0.78) | 1.40 (1.20) | 1.36 (1.23) | 1.04[f](0.83–1.29[g]) |
| $Mg(OH)_2$ surface energy | 0.50 (0.43) | 0.44 (0.14) | 0.44 (0.31) | 0.063[h] (0.053[i]) |
| Molecular adsorption energy[b] | −21.6(−21.5) | −15.4(−14.3) | −14.4(−15.2) | (−11.1 – −17.5[j]) |
| Dissociative adsorption energy[b] | −15.2(−17.1) | −14.2(−13.5) | −8.0(−10.2) | (−6.2[k]) |
| H-bond energy of water dimer | −12.0 | −4.9 | −5.0 | (−5.0[l]) |

[a] In the "ReaxFF", "DFTB", and "DFT" columns, the values outside the parentheses are calculated using the fully optimized structures with the respective method, while those in parentheses are calculated using a supercell created based on the experimental lattice parameters. The values outside (in) parentheses in the "Literature" column are the experimentally obtained (computationally estimated) values. Units are Å for length, kcal/mol for energy, and $J/m^2$ for surface energy. [b] Each row lists the molecular or dissociative adsorption energy for a single water molecule on the MgO(100) surface. [c] Ref. S9 [d] Ref. S10 [e] Ref. S11 [f] Ref. S12 [g] Ref. S13 [h] Ref. S14 [i] Ref. S15 [j] Refs. S16–S19 [k] Ref. S20 [l] Ref. S21

## 1.2 DFTB and DFT calculations for structure refinement

The interfacial structures obtained from the PS-MD simulations and the subsequent optimization calculations at the ReaxFF level were then further optimized using the DFTB method with the DFTB+ program package.[S22] We employed the DFTB3 level of theory[S23] with the 3OB-3-1 parameter set.[S24,S25] Grimme's D3 dispersion correction[S26,S27] was included, as dispersion forces are known to be important for the structure of liquid water.[S28] All DFTB calculations were performed at the Γ-point. The results of the validation calculations for the DFTB method are summarized in Table S1. The structures found to be more stable than the initial (reactant) one at the DFTB level were subjected to further refinement by DFT optimization calculations performed with the Quantum Espresso program package.[S29] We adopted the BLYP exchange-correlation functional, which is widely used and known to perform well for hydrogen-bonded systems.[S20,S30] The D3 dispersion correction and Γ-point sampling were used, consistent with the DFTB calculations. An effective screening medium (ESM) method was used to treat the open boundary condition in the $z$ direction.[S31] Norm-conserving and ultrasoft pseudopotentials were used for Mg and for O and H, respectively. After convergence tests, the kinetic energy cutoff for the plane-wave basis set and the charge density cutoff were set to 30 Ry and 300 Ry, respectively. These cutoffs ensure high accuracy, with errors in the MgO and $Mg(OH)_2$ lattice constant parameters below 0.01 Å and the hydration reaction energy below 0.2 kcal/mol compared to the calculations with a 300 Ry cutoff for the kinetic energy. At the DFT level, we employed a two-step refinement procedure. First, optimizations were performed on all promising DFTB structures using loose convergence criteria of $5.0\times10^{-4}$ Hartree for energy and $5.0\times10^{-3}$ Hartree/Bohr for its gradient. This step was used to efficiently screen for stable structures. Second, the structures found to be more stable than the initial (reactant) one in the first step were re-optimized using convergence criteria that were one order of magnitude tighter ($5.0\times10^{-5}$ Hartree and $5.0\times10^{-4}$ Hartree/Bohr for energy and its gradient, respectively) for detailed analysis (Section 3 in the main text).

## 1.3 Simulation system and conditions

We used the same simulation model across all three computational levels (ReaxFF, DFTB, and DFT) to ensure consistency. The system consisted of a five-layer MgO slab with the (100) surface exposed to a vacuum. While other facets or steps may facilitate hydration,[S32–S34] the ideal (100) surface was chosen to gain fundamental insights into the hydration processes, since this is the most thermodynamically stable facet in a vacuum. The supercell had lateral dimensions of 16.85 Å $\times$ 16.85 Å, constructed based on the experimental lattice constant of MgO (4.21 Å)[S9] to provide a unified basis for the different computational levels. This choice is justified by the results in Table S1. A supercell of this size contains 32 MgO pairs per layer. Test calculations with a larger (e.g., 3$\times$3) supercell confirmed that these lateral dimensions are sufficient to yield consistent PS-MD results. Two monolayers (ML) of water, corresponding to a total of 64 water molecules, were placed on the MgO slab. This two ML coverage represents a high-humidity environment (RH > $\sim$70%) and is considered the minimum for observing $Mg^{2+}$ dissolution and subsequent hydration based on experimental findings.[S35] From a stoichiometric perspective, at least two ML of water are also required for the subsurface MgO layers to react. The simulation cell size in the $z$ direction was set to 60 Å for the ReaxFF and DFTB calculations and 45 Å for the DFT calculations to ensure a sufficient vacuum region. The bottom two layers of the MgO slab were fixed at their bulk crystal positions in the optimization calculations.

The hydration of MgO has been investigated under various surface (e.g., facets and defects) and environmental (e.g., pH, humidity, temperature, and pressure) conditions, which have been shown to intricately affect the reaction kinetics.[S32,S36–S40] In contrast, this study focuses on the reaction process occurring at the MgO/water interface at room temperature, specifically on an isolated, perfect surface with two adsorbed water layers. It is well-known, not only for the present system[S34,S41,S42] but also for other systems,[S43–S45] that the presence of defects can facilitate the reaction. In addition, it is experimentally known that a high pH, corresponding to an abundance of $OH^-$ ions, promotes the nucleation of $Mg(OH)_2$.[S37] Furthermore, although the two-layer water film on the MgO surface represents a relatively high-humidity environment,[S35] the adsorption of

additional water molecules onto $Mg^{2+}$ ions in the gas-liquid interface is not considered in this study. Therefore, the present calculations correspond to an inert condition relative to the more complex conditions found in many experiments. For example, with a continuous supply of water molecules, we might observe a more extensive $Mg^{2+}$ dissolution than shown in the main text. This focus on an idealized system provides a crucial foundation for understanding the intrinsic hydration process. The results serve as a point of comparison for evaluating the actual hydration reaction, where various factors such as defect formation, high pH, and a continuous water supply are intricately interrelated. By comparing with the present results, the contribution of each factor to the reaction mechanism and kinetics can be systematically evaluated in future work.

## 1.4 NEB calculations for $Mg^{2+}$ dissolution

As described in the main text, we selected the final configurations of the first stage, which represented local energy minima, as the reactant states for nudged elastic band (NEB) calculations. The product structure, formed when each $Mg^{2+}$ ion dissolved, was determined through a multi-step procedure. The procedure was initiated from a reactant structure. First, we displaced a dissolving $Mg^{2+}$ ion by 0.2 Å in the positive $z$ direction. This displaced geometry was then used as the initial structure for a constrained optimization, in which the $z$ coordinate of the $Mg^{2+}$ ion was held fixed. This displacement-then-optimization procedure was repeated for subsequent steps: the $Mg^{2+}$ ion in the previously optimized structure was moved by an additional 0.2 Å, followed by another constrained optimization. This iterative procedure was finished when the $Mg^{2+}$ion reached a final $z$ coordinate of 2.6 Å. Next, the most stable structure in the $z$ = 2.2 Å – 2.6 Å range was subjected to an unconstrained geometry optimization. The final resulting structure was designated as the product state if it represented a local energy minimum with the final $z$ coordinate of the $Mg^{2+}$ ion being greater than 0.75 Å.

We used the Quantum Espresso program package for the NEB calculations. Ten intermediate images were generated to connect the reactant and product structures. The spring constant parameters, $k_{\mathrm{min}}$ and $k_{\mathrm{max}}$, which are used in Quantum Espresso, were set to 0.4 and 0.6 Hartree/Bohr$^2$, respectively. The reaction path was considered converged when the maximum force component orthogonal to the path fell below 0.003 Hartree/Bohr. All other DFT parameters were the same as those described in Section 1.2 in Supporting Information.

## 1.5 PS-MD simulations for nucleation in water

To observe the nucleation of $Mg(OH)_2$ in bulk water, an environment far from the MgO surface and abundant in water molecules, we performed additional PS-MD simulations. The simulation system was constructed as follows. We began by taking the final snapshot from the 1,000th PS-MD cycle of the PS-MD simulation performed for structure generation. From this snapshot, we extracted the amorphous phase comprising Mg, O, and H atoms that had formed above the MgO surface (defined as a $z$ coordinate > $\sim$2 Å). The structure from the 1,000th PS-MD cycle was intentionally chosen to ensure a higher concentration of dissolved $Mg^{2+}$ ions within the amorphous system. While the most potential-energetically favorable interface structures were typically formed by approximately the 300th PS-MD cycle, it is rational to consider that $Mg^{2+}$ dissolution would persist with a sufficient supply of water. Thus, using the 1,000th PS-MD cycle structure is a consistent approach for this purpose. This extracted amorphous phase was then solvated in a bulk water box. The lateral (*xy*) dimensions of the new simulation box were maintained at 16.85 Å $\times$ 16.85 Å, identical to those of the original MgO/water slab system. The box length in the $z$ direction was determined using an *NPT* ensemble simulation (300 K and 1 atm). The resulting final system contained approximately 45 Mg, 310 O, and 530 H atoms. Although this system corresponds to a very high Mg concentration of 9-10 mol/L, we believe that such a value can be plausible by considering a transient concentration of $Mg^{2+}$ ions dissolved in a thin water film formed under high-humidity conditions. Using such newly prepared system, we then performed PS-MD simulations. The computational parameters were identical to those used in the main PS-MD simulations for structure generation, with the exception of the potential scaling factor, $\alpha$. Based on preliminary calculations, we set $\alpha$ to 0.9991. This is because we found that the original value ($\alpha$ = 0.999) used for structure generation in the MgO/water slab system flattened the potential energy surface too aggressively, which hindered the necessary aggregation of $Mg^{2+}$ ions for nucleation.

# 2 Potential Energy Variation of Interfacial Structures

Here, we discuss the potential energy variation accompanying the interfacial structural changes depicted in Figure 1 in the main text. Figure S2 shows the potential energy variation, and the green circles indicate the potential energy of the six interfacial structures depicted in Figures 1a-f. The interfacial structures generated throughout the present procedure (described in Sections 1.1 and 1.2 in Supporting Information) are found to be comparable to, or even more stable than, the initial one. Although the potential energy varies among the structures, its variation is qualitatively consistent with the exothermic nature of the hydration reaction of MgO. Some of the structures obtained by the calculations are stabilized by about 100 kcal/mol from the initial structure, which indicates a stabilization of $\sim$1.5 kcal/mol per water molecule by the interfacial hydration reaction. On the other hand, the adsorption process prior to the interfacial chemical reaction was found to stabilize the system by $\sim$16.5 kcal/mol per water molecule, with respect to the state of the perfect MgO slab and 64 isolated water molecules. (Giordano and co-workers have reported the stabilization by adsorption of a water monolayer to be 13.9 kcal/mol,[S46] which is comparable to our calculations.) Thus, the partly hydrated states obtained by the present calculations are stabilized by a maximum of $\sim$18 kcal/mol per water molecule, compared to the state consisting of the MgO slab and the isolated water molecules in the gas phase. Based on the reaction energy of $\sim$28 kcal/mol calculated with the slab geometries of MgO and $Mg(OH)_2$, our calculation indicates that a $\sim$64% hydration reaction has been achieved in terms of potential energy. (The reaction energy with the bulk geometries of MgO and $Mg(OH)_2$ is $\sim$19 kcal/mol as shown in Table S1.) The results for the other four runs are separately summarized in Figure S5. We note that fewer and less stable structures are screened after the $\sim$400th PS-MD cycle. This is due to the difference in accuracy between the ReaxFF method used in the PS-MD simulation and the DFTB/DFT methods used in the structure refinement (Figure S3).

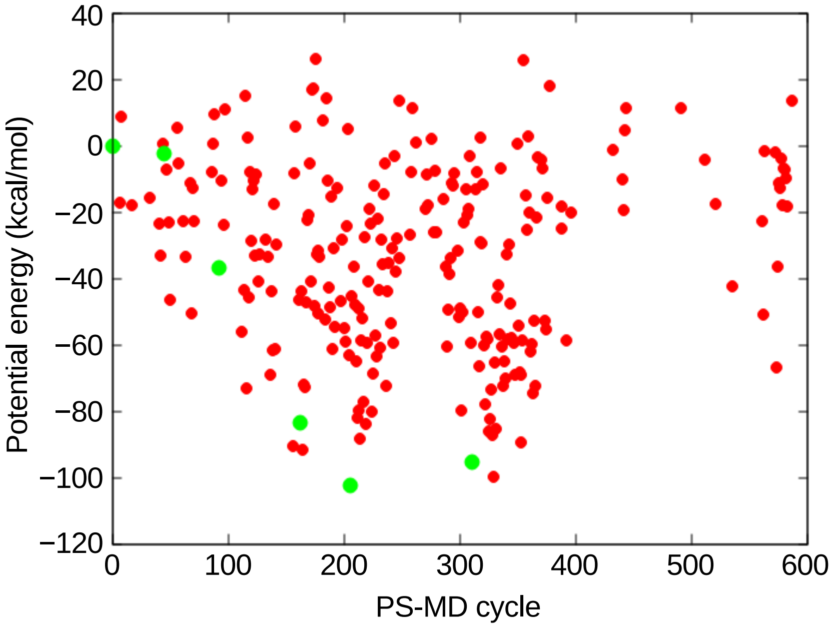


Figure S2: Potential energy variation (kcal/mol) of the MgO/water interface structures along the PS-MD cycle. The potential energies are calculated in the second step of the DFT-level optimizations. The green circles indicate the potential energies of the structures shown in Figure 1 in the main text. The potential energy at the initial PS-MD cycle is set to zero as a reference. The potential energies of the discarded structures prior to the second step of the DFT-level optimization are not shown.

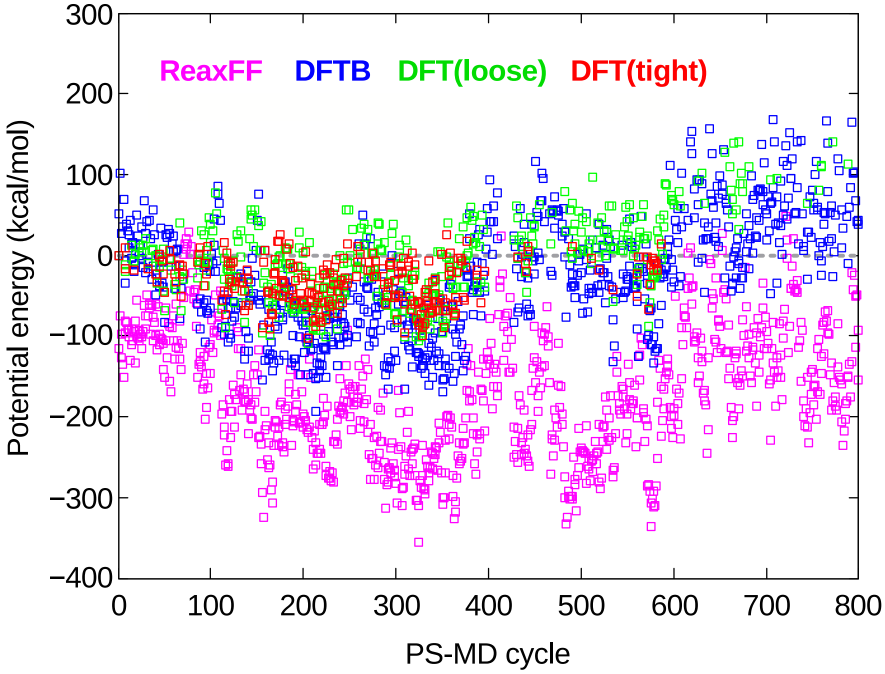


Figure S3: Variation in potential energy of the MgO/water interface structures optimized at each level of theory along the PS-MD cycle. The relative energy variations are roughly similar among the three levels of theory, validating the step-by-step structure screening approach employed here. The observation of many structures more stable than the initial one indicates that the simulation successfully traced the exothermic hydration process. Furthermore, after the ∼300th PS-MD cycle, new stable structures are rarely found at the DFT level with the tight convergence criteria, which suggests that only the structures obtained up to this point are suitable for structural analysis.

# 3 Supplementary Tables and Figures

Table S2: PS-MD Cycle Range in the Five Independent Runs Used to Examine MgO/water Interfacial Structures in Section 3.3 in the Main Text and the Number of $Mg^{2+}$ Ions Dissolved from the MgO Surface ($N_{Mg^{2+}}$) in the Range.

| Run[a] | PS-MD cycles | $N_{Mg^{2+}}$ |
|---|---|---|
| A | 16 – 64 | 11 |
| B | 43 – 102 | 8 |
| C | 33 – 114 | 13 |
| D | 19 – 60 | 8 |
| E | 41 – 112 | 12 |

[a] Run E corresponds to the run used in Section 3.1 in the main text.

(A)

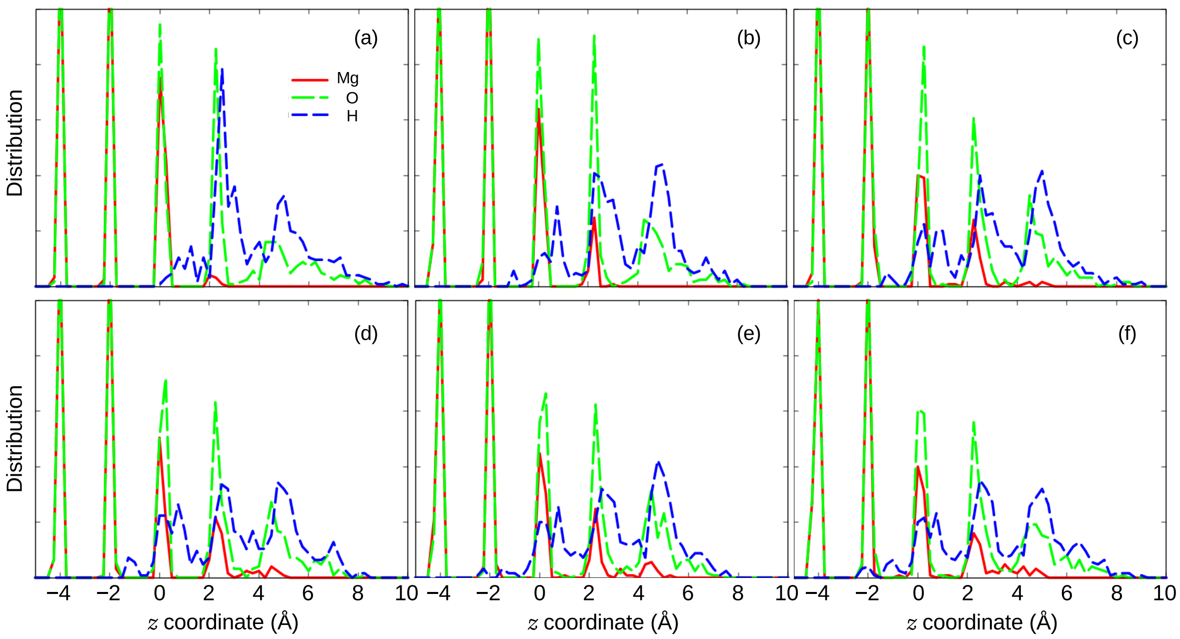
(a)
(b)
(c)
(d)
(e)
(f)
Mg
O
H
Distribution
Distribution
−4 −2 0 2 4 6 8 10
z coordinate (Å)

(B)

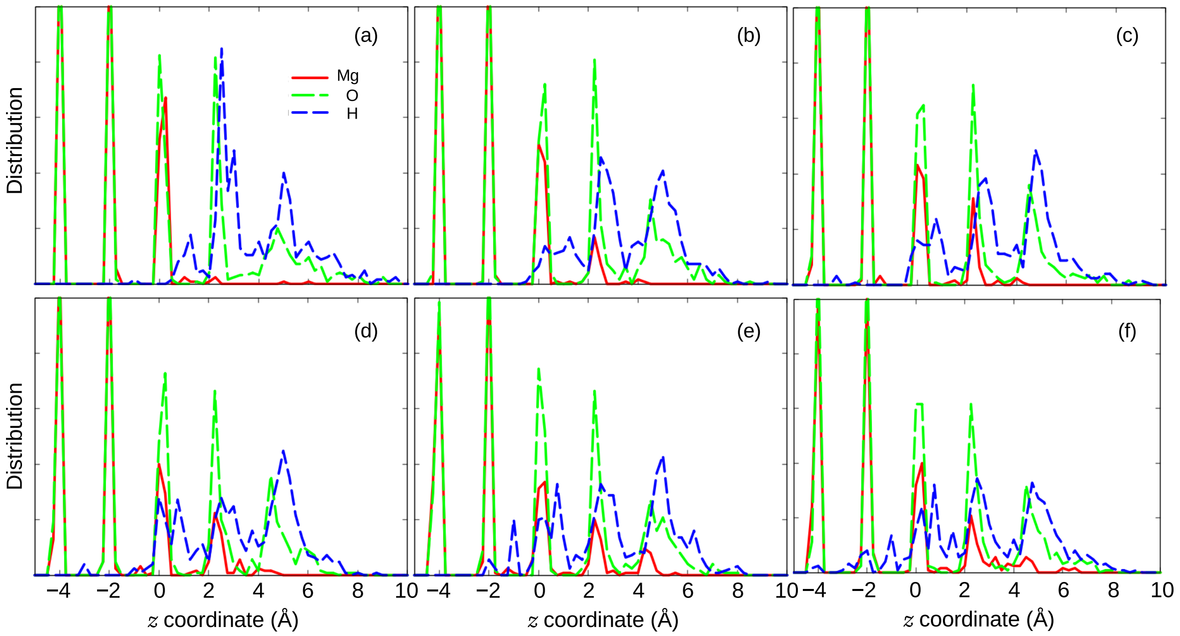
(a)
(b)
(c)
(d)
(e)
(f)
Mg
O
H
Distribution
Distribution
−4 −2 0 2 4 6 8 10
z coordinate (Å)

(C)

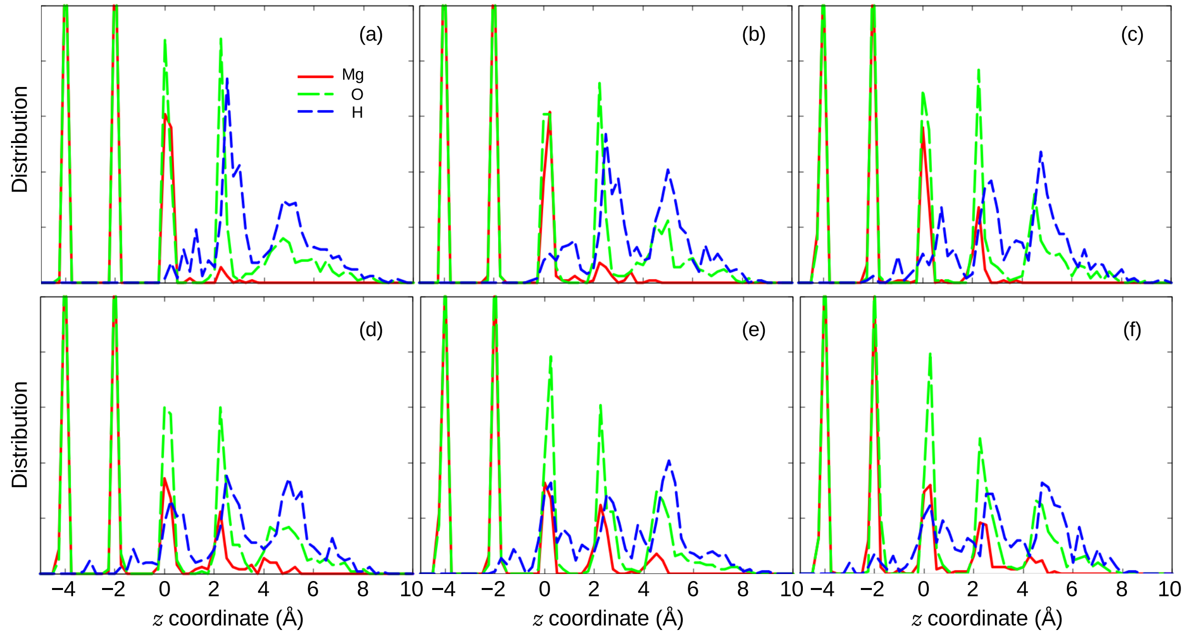


(D)

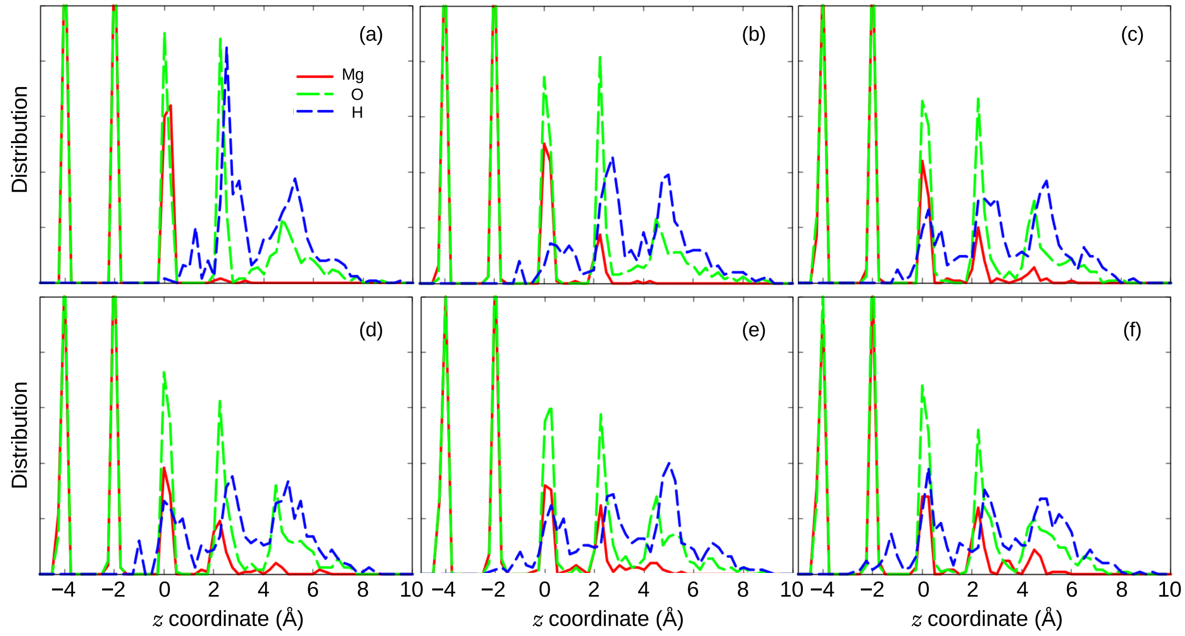


Figure S4: Distribution of the $z$ coordinates of Mg (red), O (green), and H (blue) atoms with respect to the PS-MD cycle obtained from the four independent runs (A-D) not presented in the main text. The distributions in panels (a)-(f) are averaged over five configurations from specific PS-MD cycle ranges for each simulation: (A) 0-20, 51-57, 86-114, 148-152, 194-200, and 273-303; (B) 0-57, 100-105, 148-152, 190-209, 263-268, and 379-391; (C) 0-37, 50-56, 90-106, 154-159, 197-201, and 281-296; and (D) 0-20, 51-57, 97-104, 148-153, 194-207, and 274-293.

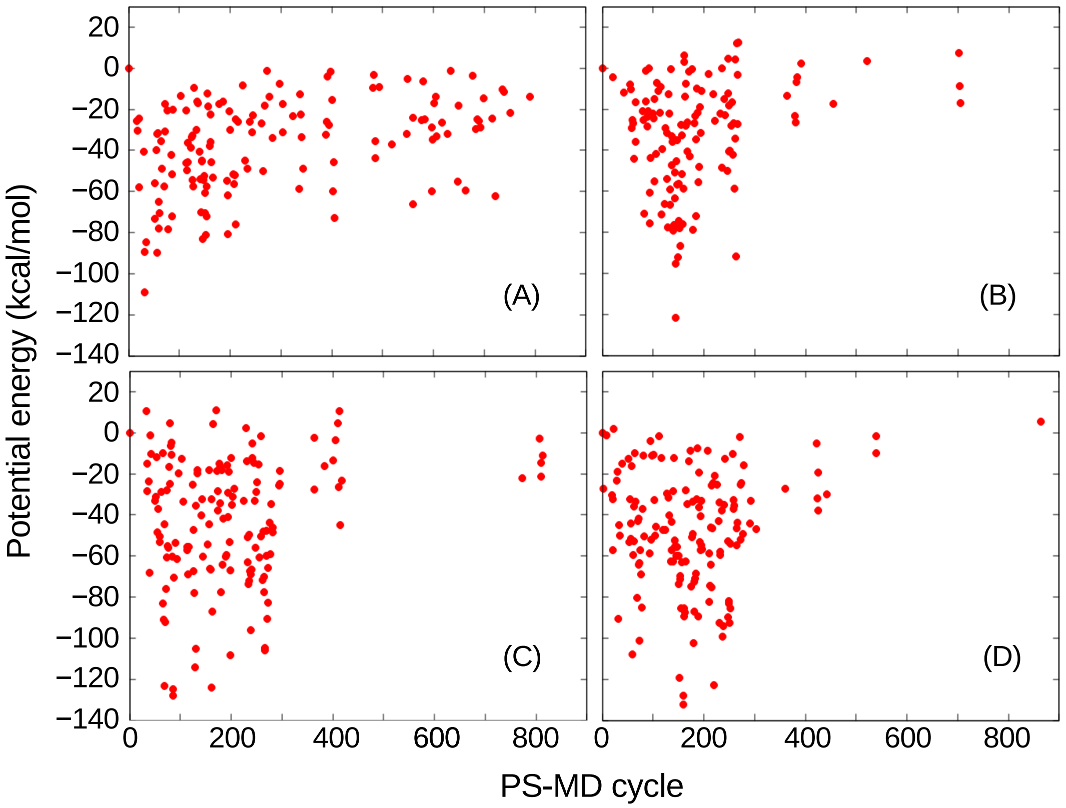


Figure S5: Potential energy variation (kcal/mol) of the MgO/water interface structures along the PS-MD cycle calculated from the four independent runs not presented in the main text. The energy variation corresponding to the run used in the main text is shown in Figure S2. The potential energies are calculated in the second step of the DFT-level optimizations. The potential energy at the initial PS-MD cycle is set to zero as a reference in each plot. Each panel, (A) through (D), corresponds to one of the four independent runs referenced in Figure S4.

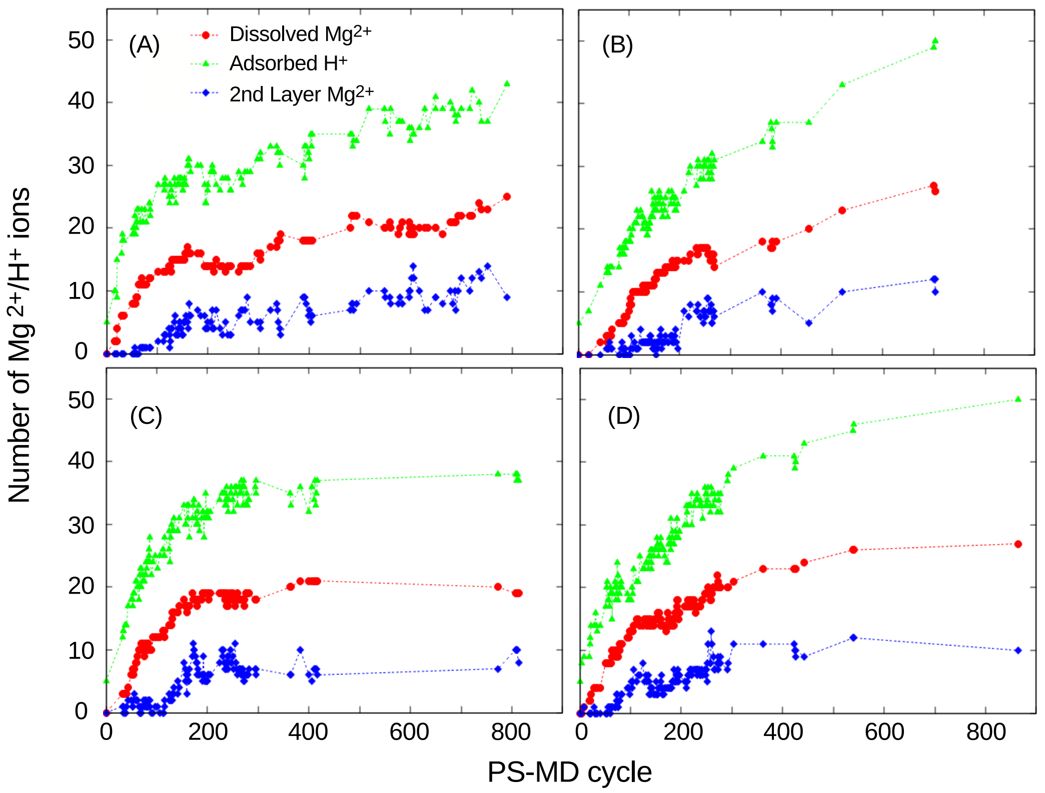


Figure S6: Number of dissolved $Mg^{2+}$ ions (red) and adsorbed/penetrated protons (green) along the PS-MD cycle, calculated from the four independent runs not presented in the main text. The number of $Mg^{2+}$ ions in the second water layer, whose $z$ coordinates are higher than 2.75 Å, is also shown in blue. Each panel, (A) through (D), corresponds to one of the four independent runs referenced in Figure S4.

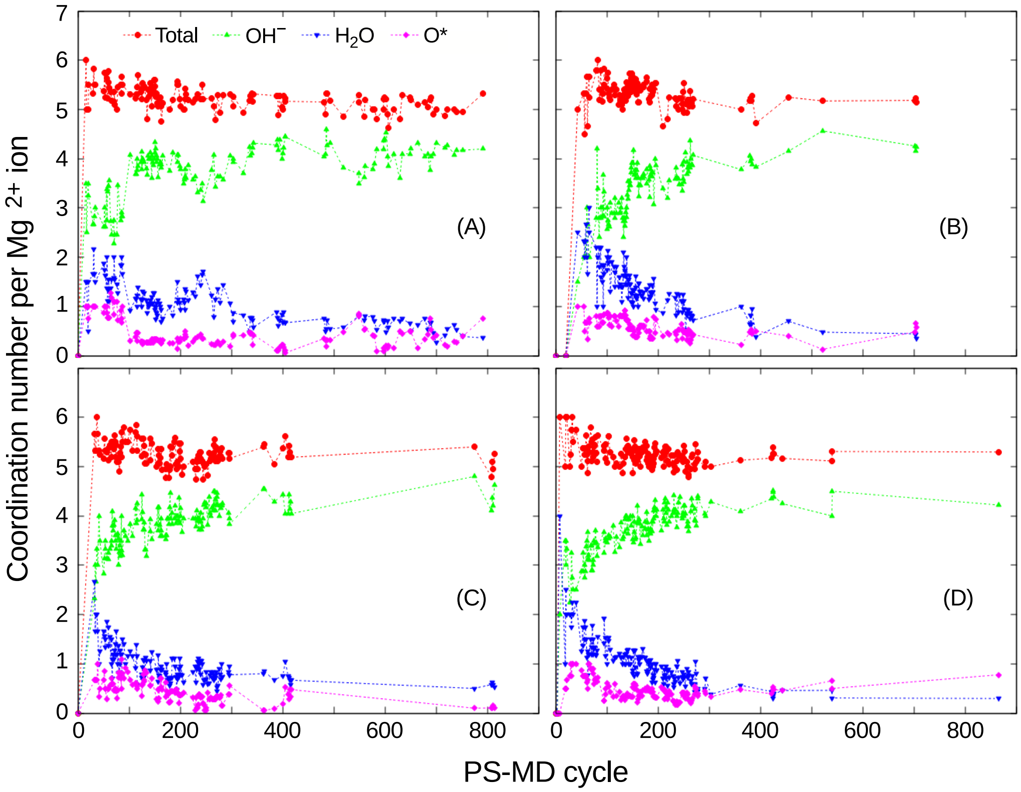


Figure S7: Coordination number per $Mg^{2+}$ ions along the PS-MD cycle, calculated from the four independent runs not presented in the main text. The total coordination number is shown in red. Contributions to the coordination number from $OH^-$ (green), $H_2O$ (blue), and MgO surface oxygen atoms (O*; magenta) are also shown. Each panel, (A) through (D), corresponds to one of the four independent runs referenced in Figure S4.

(A)

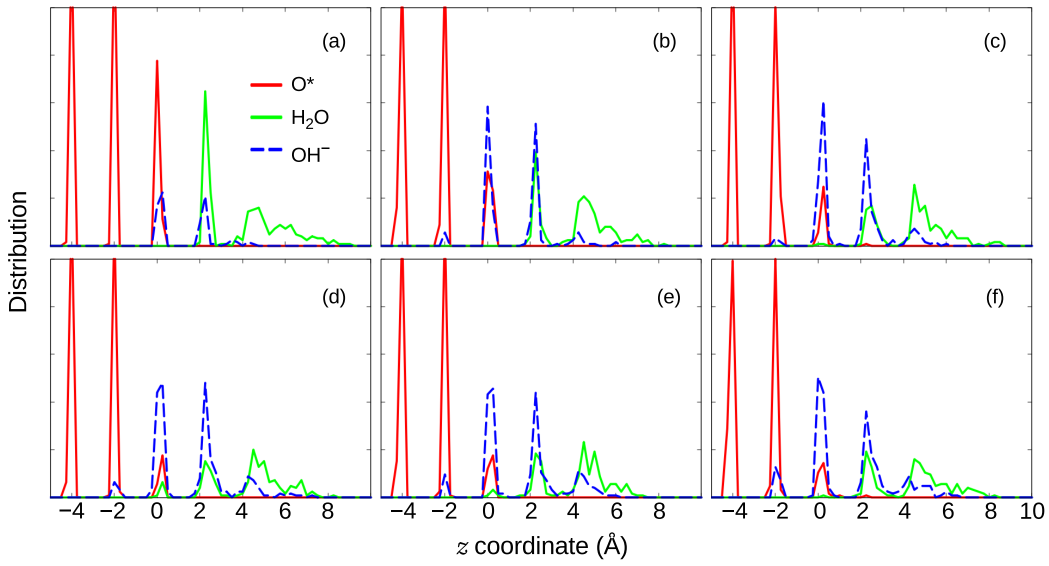

(a)
(b)
(c)
(d)
(e)
(f)
O*
$H_2O$
$OH^-$
Distribution
−4 −2 0 2 4 6 8 10
z coordinate (Å)


(B)

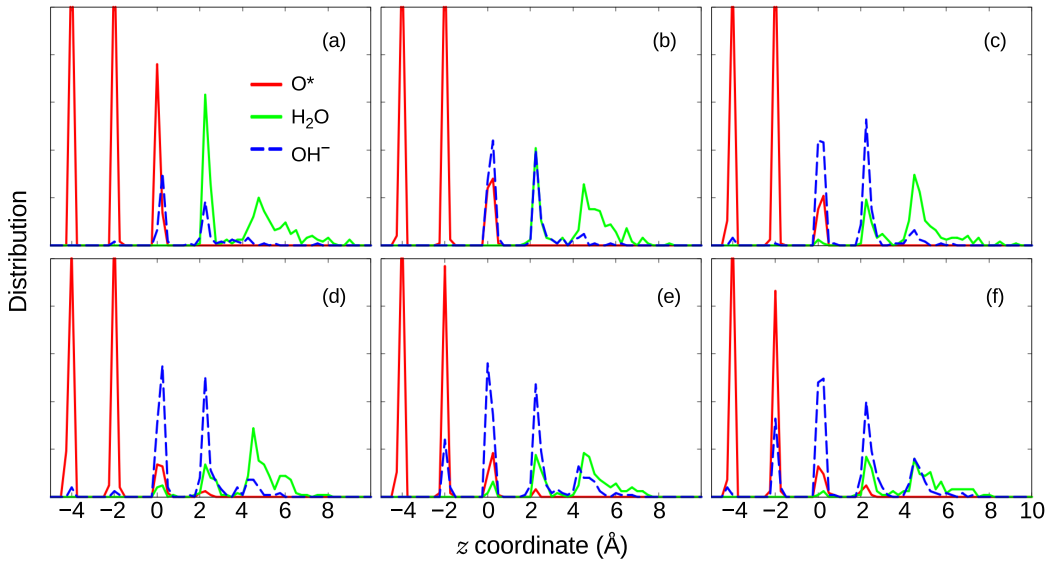

(a)
(b)
(c)
(d)
(e)
(f)
O*
$H_2O$
$OH^-$
Distribution
−4 −2 0 2 4 6 8 10
z coordinate (Å)

(C)

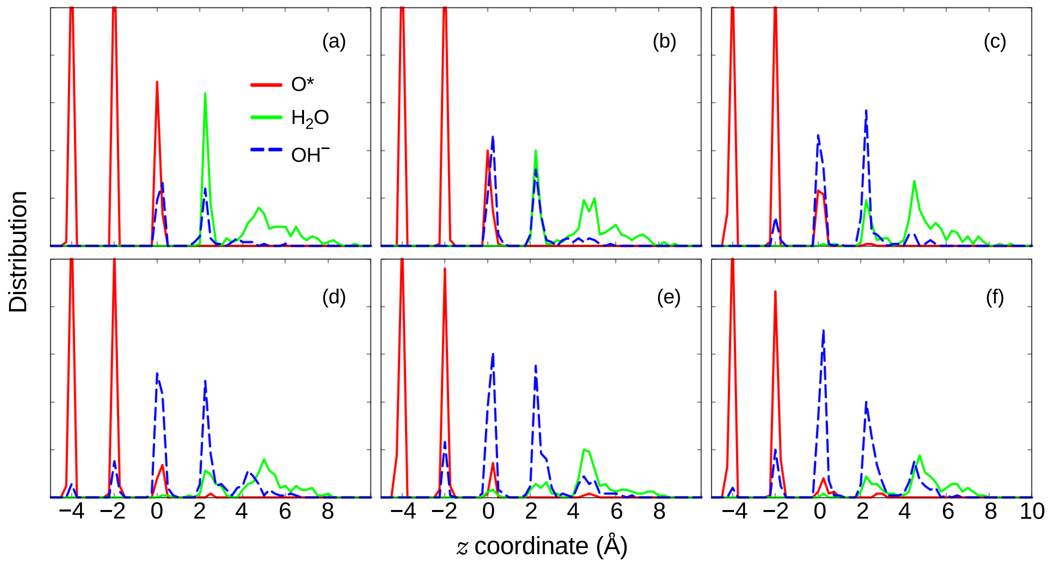

(a)
(b)
(c)
(d)
(e)
(f)
O*
H2O
OH⁻
Distribution
−4 −2 0 2 4 6 8 10
z coordinate (Å)


(D)

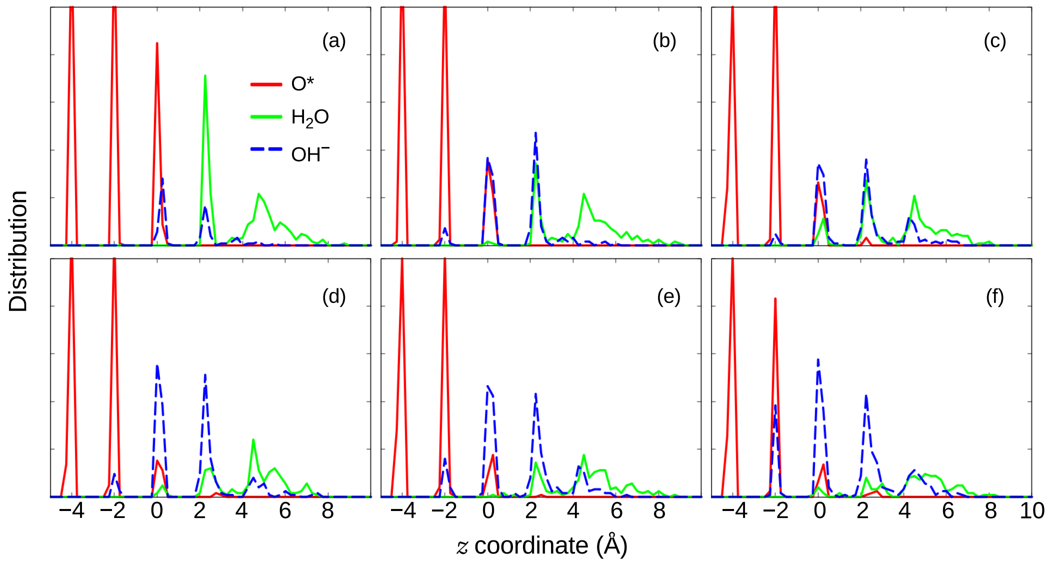

(a)
(b)
(c)
(d)
(e)
(f)
O*
H2O
OH⁻
Distribution
−4 −2 0 2 4 6 8 10
z coordinate (Å)

(E)

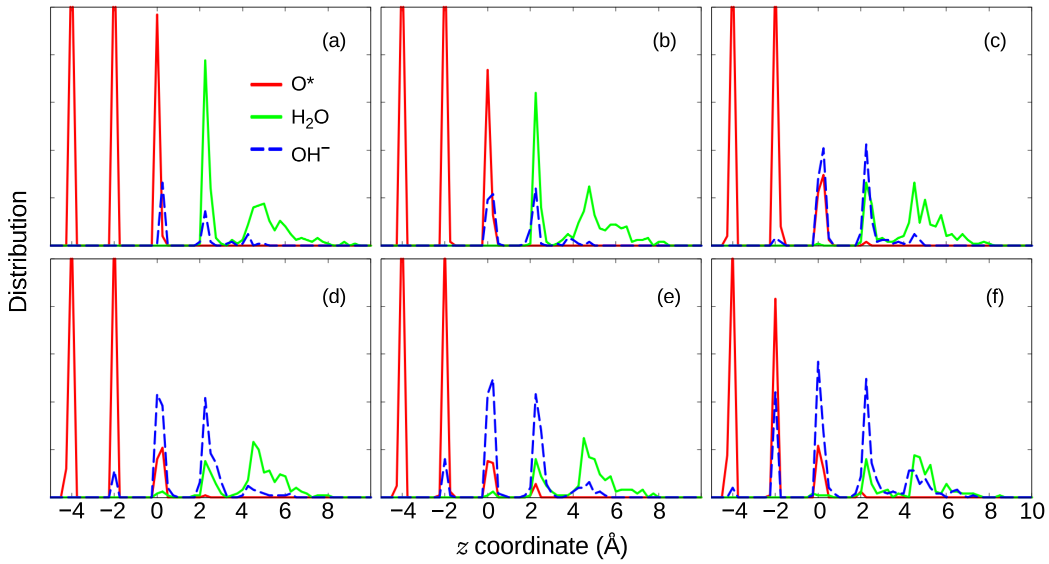


Figure S8: Distribution of the $z$ coordinates of oxygen atoms in $O^*$ (red), $H_2O$ (green), and $OH^-$ (blue) groups with respect to the PS-MD cycle. Panels (A-D) correspond to the runs shown in Figure S4, while panel (E) corresponds to the run shown in Figure 1 in the main text. The configurations used in respective panels are also the same as those in Figure S4 and Figure 1.

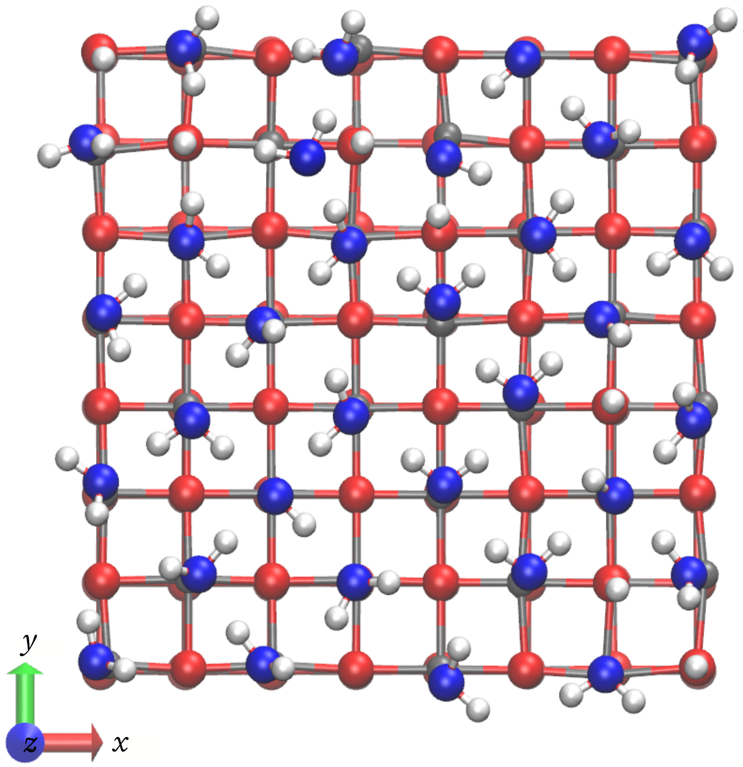


Figure S9: Top view of a typical MgO/water interfacial structure in the first stage of the hydration process. Mg, O, and H atoms are colored gray, red, and white, respectively, except for the oxygen atoms in the water layer, which are colored blue. The water molecules in the second layer on the gas phase are not shown. The observation that the oxygen atoms of the water molecules on the MgO surface reside atop Mg* atoms is consistent with the MD simulation results by McCarthy and co-workers.[S16]

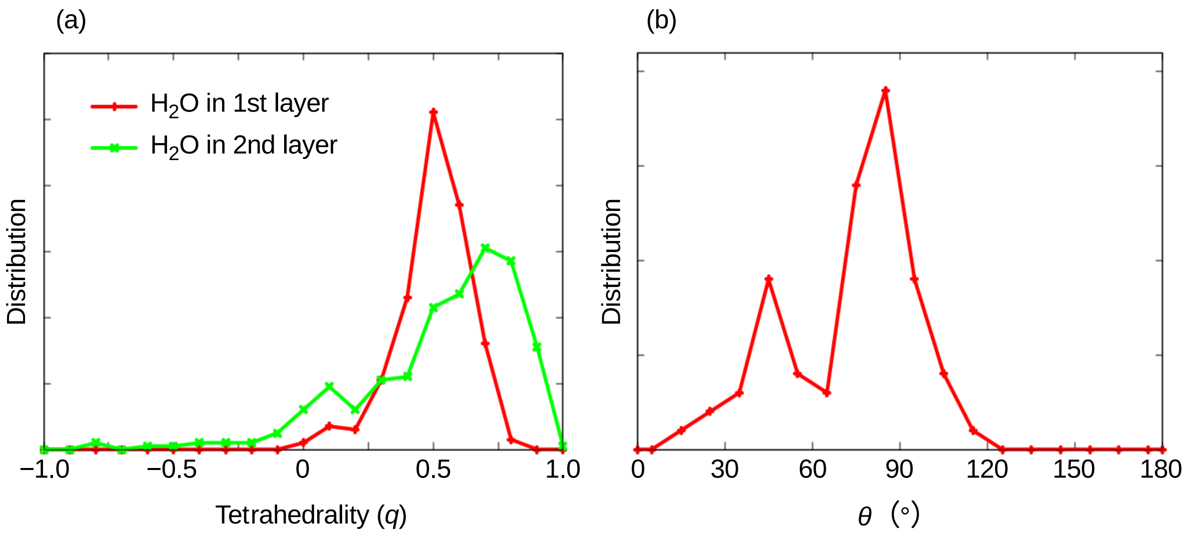


Figure S10: (a) Distribution of the tetrahedral order parameter (or tetrahedrality; $q$) of the water molecules in the first (red) and second (green) layers. The parameter $q$ is calculated according to the method in Ref. S47. For comparison, the distribution for bulk water exhibits a prominent peak at $q \sim 0.75$ and a shoulder at $q \sim 0.5$, but lacks a long tail for $q < 0$.[S47] These latter features arise from a disordered local structure in the HB network. The $q$ distributions for the water molecules in the layers are clearly distinct from that of bulk water, indicating a different structural arrangement. (b) Distribution of the angle $\theta$ between the dipole moment vector of an $OH^-$ ion in the first water layer and the $z$ axis. These distributions are calculated using the interfacial structures observed in the first stage of the hydration process.

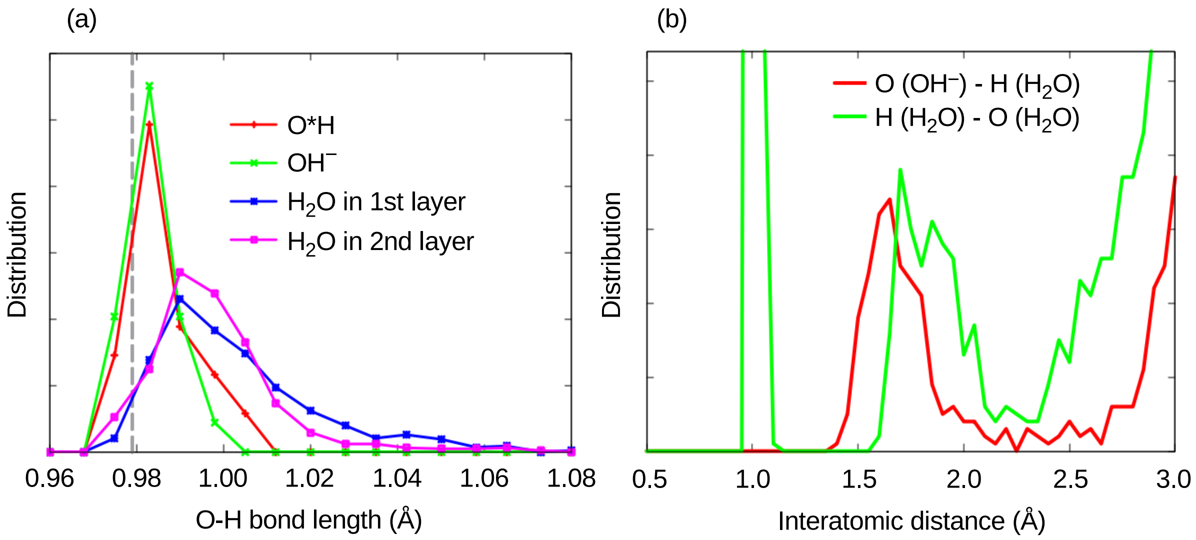


Figure S11: (a) Distribution of the O-H bond length in O*H (red), $OH^-$ (green), $H_2O$ in the first layer (blue), and $H_2O$ in the second layer (magenta). (b) Radial distribution function between the O atom of an $OH^-$ ion and the H atom of an $H_2O$ molecule (red) and between the H atom of one $H_2O$ molecule and the O atom of another (green). The gray dashed line in panel (a) represents the O-H bond length of the isolated water molecule. These distributions are calculated using the interfacial structures observed in the first stage of the hydration process.

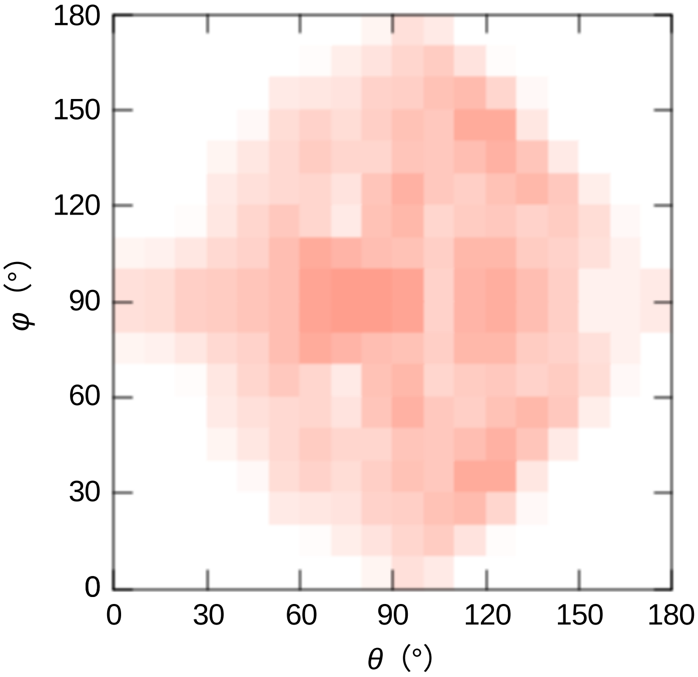


Figure S12: Two-dimensional probability distribution of the orientation angles $\theta$ (°) and $\varphi$ (°) for water molecules in the second layer. A darker color indicates higher probability. The definitions of the angles $\theta$ and $\varphi$ are the same as described in the main text.

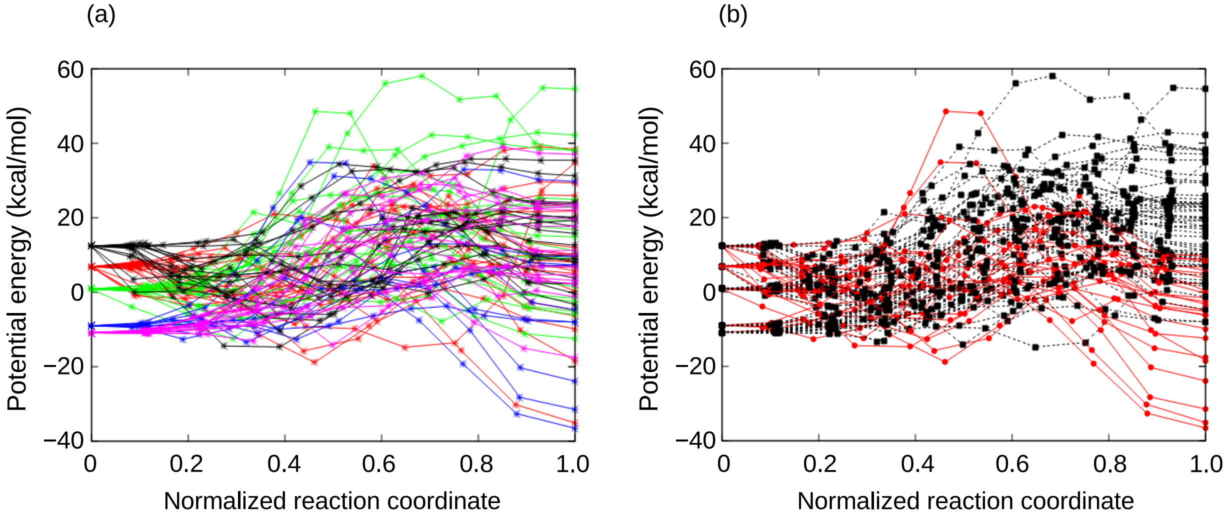


Figure S13: Potential energy profile of the $Mg^{2+}$ dissolution process calculated by the nudged elastic band (NEB) method at the DFT level. A total of 83 profiles resulting in a locally stable product structure (i.e., $Mg^{2+}$-dissolved structure) are shown, colored according to the individual PS-MD simulation run in (a) and by the reaction energy in (b). In panel (b), the reaction profiles with negative and positive reaction energies are colored red and black, respectively. In both panels, the potential energy reference is set to the average energy of the five reactant structures.

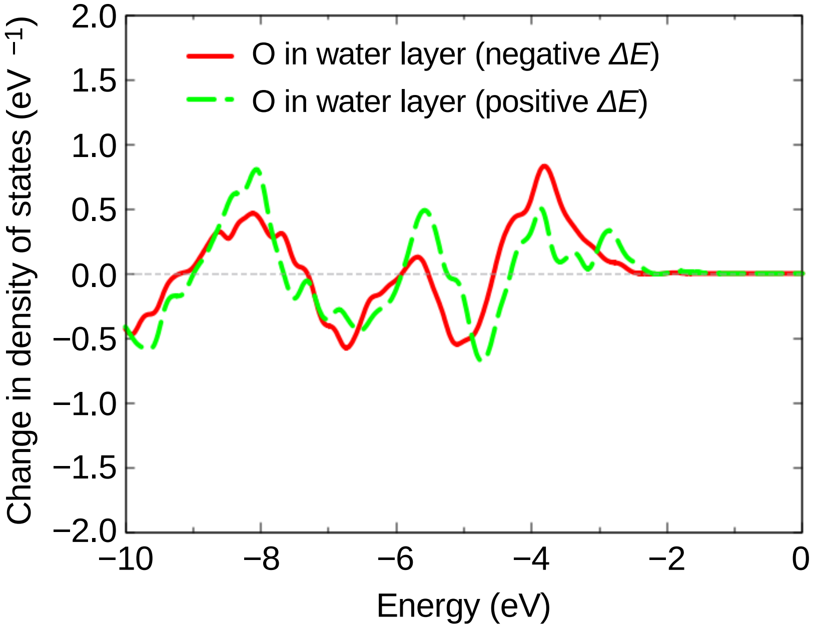


Figure S14: Change in the projected density of states (pDOS) of the O atoms coordinating to a dissolved $Mg^{2+}$ ion in the water layer for the dissolution process. The pDOS changes for the processes with negative and positive reaction energies ($\Delta E$) are colored red and green, respectively. The reference energy is set to the vacuum level in the slab model. The minor difference observed between the red and green lines is likely caused by variations in the water layer structure and, in part, by insufficient sampling of the O atoms. Thus, the effect of the electronic structure of the water layer on the dissolution reaction energy is considered to be small. This observation is consistent with the result that the coordination number of $H_2O$ and $OH^-$ to a dissolved $Mg^{2+}$ ion has a less significant effect on the reaction energy than does the number of protonated $O^*$ atoms (Figure 5 in the main text).

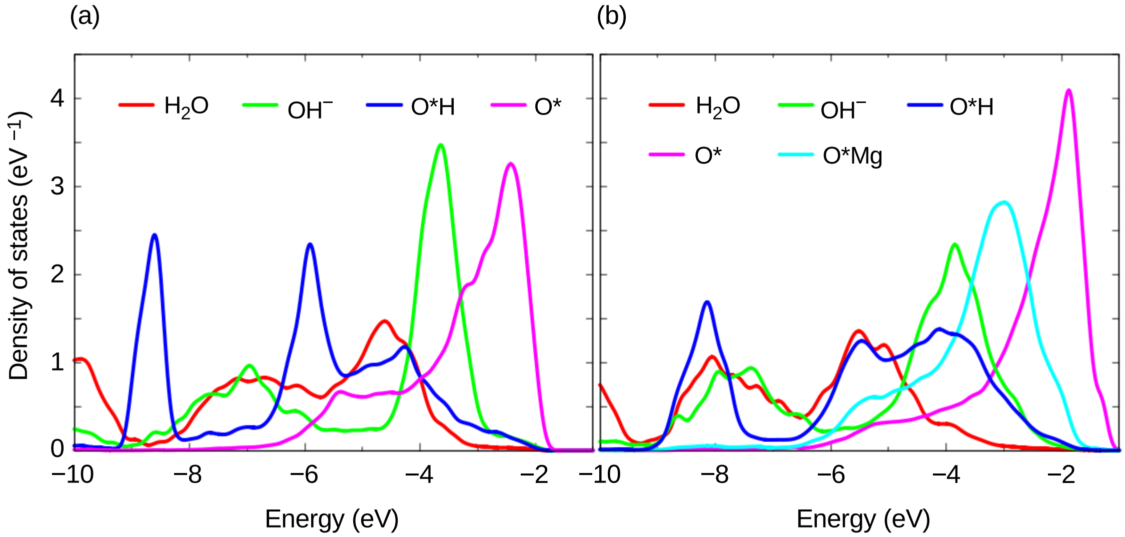


Figure S15: Projected density of states (pDOS) of oxygen atoms in the reactant (a) and product (b) states. The oxygen atoms are classified into five types: water molecule ($H_2O$, red), hydroxide ion ($OH^-$, green), proton-adsorbed surface oxygen atom ($O^*H$, blue), intact surface oxygen atom ($O^*$, magenta), and surface oxygen atom coordinating to a dissolved $Mg^{2+}$ ion ($O^*Mg$; cyan). Note that the water molecules and the hydroxide ions used in panel (b) are coordinated to a dissolved $Mg^{2+}$ ion. In panel (a), the Mg-O bonding interaction in the MgO surface is observed as the shoulder peaks at $-5.5$ and $-3.3$ eV in the pDOS of intact surface oxygen atoms. In panel (b), the coordination of water molecules and hydroxide ions to a dissolved $Mg^{2+}$ ion gives rise to the broad peak at approximately $-8$ eV. In addition, the broad peak for $O^*H$ in the range of $-6$ to $-3$ eV in panel (b) is partly attributed to a change in $O^*$ state (i.e., protonation) during the $Mg^{2+}$ dissolution processes with a negative reaction energy.

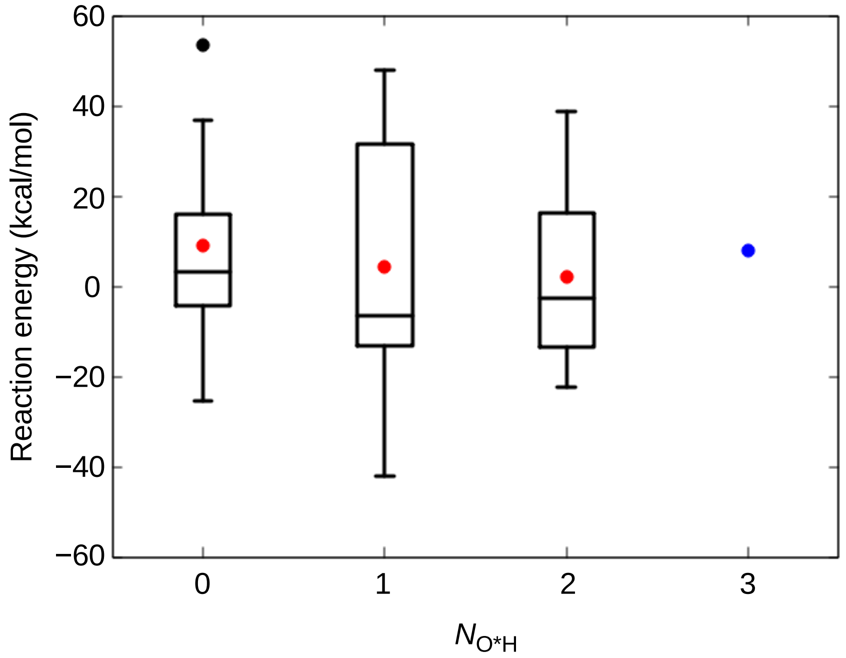


Figure S16: Boxplot of the reaction energy (kcal/mol) for the $Mg^{2+}$ dissolution process. The data are classified by $N_{O^*H}$, the number of hydroxylated $O^*$ atoms surrounding the dissolving $Mg^{2+}$ ion in the initial reactant configuration.

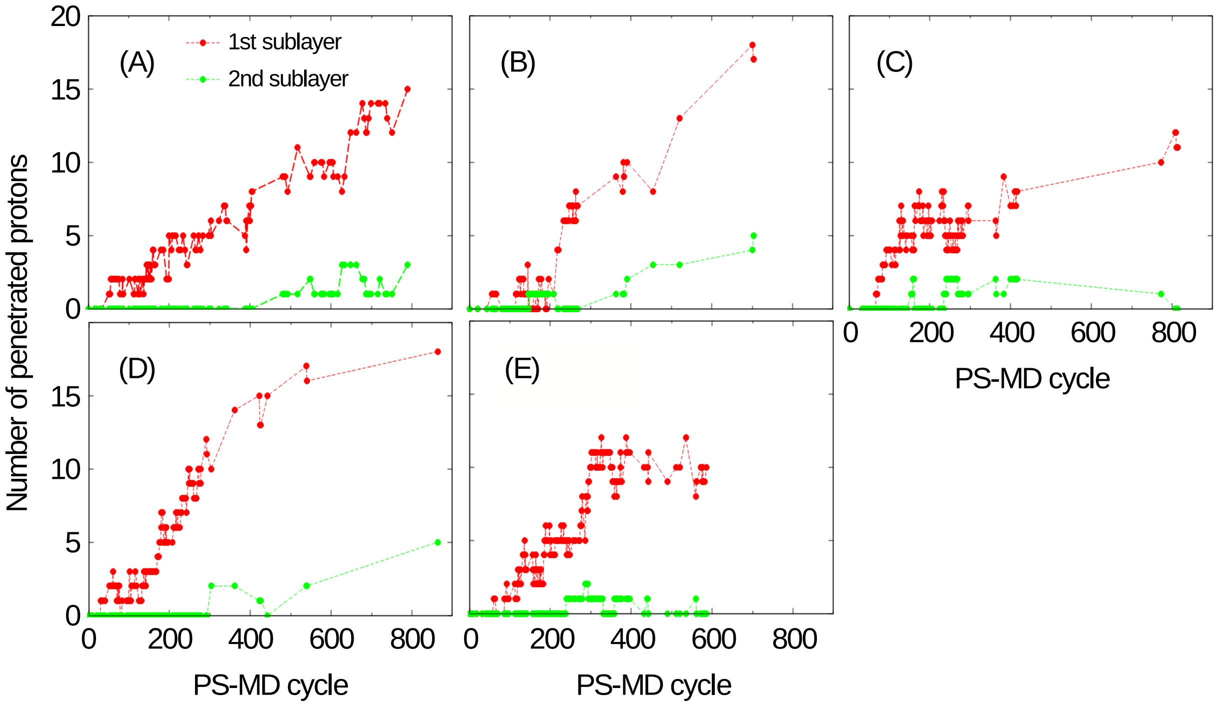


Figure S17: Variation of the number of protons penetrated into the MgO solid along the PS-MD cycle. Each panel (A-E) corresponds to the respective panel in Figure S8. The red and green circles represent the number of protons bonded to oxygen atoms in the first and second sublayers of MgO, respectively. The dashed lines are guides for the eye.

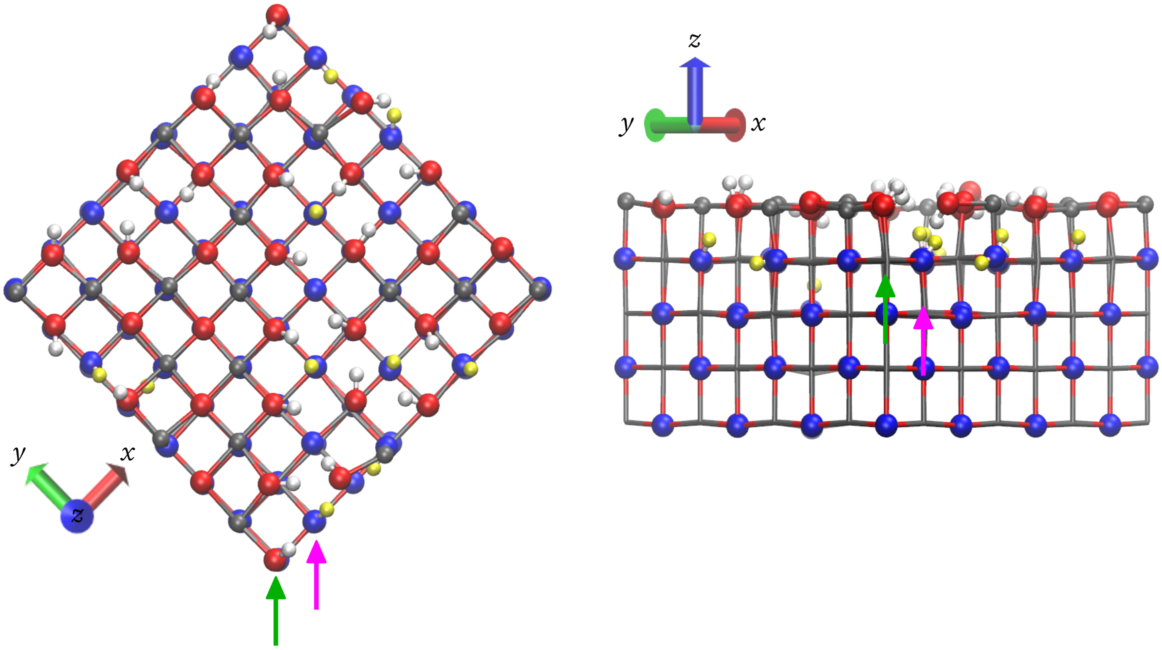


Figure S18: Top (left) and side (right) views of a characteristic MgO/water interface in the third stage of the hydration process. The $OH^-$ rows along the [110] direction can be found on the surface and in the first sublayer, as represented by the green and magenta arrows, respectively. The atoms in the water layers are omitted for clarity. Mg, O, and H atoms on the MgO surface are colored gray, red, and white, respectively. O and H atoms below the surface are colored blue and yellow, respectively.

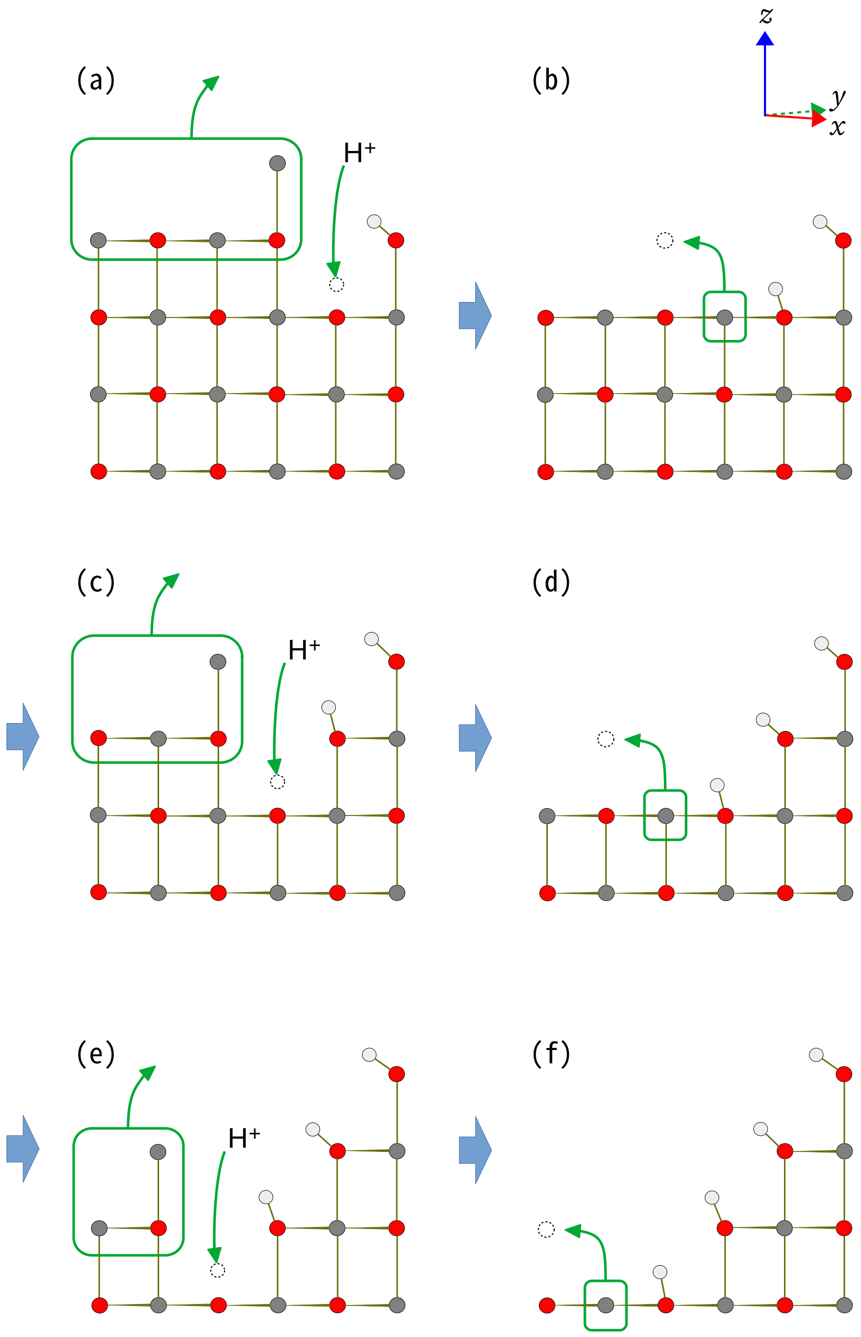


Figure S19: Schematic illustration of the nucleation process on the MgO (100) surface, starting from an $Mg^{2+}$-dissolved state. (a) The upper terrace is dissolved, followed by hydroxylation of the exposed surface oxygen atom. (b) An $Mg^{2+}$ ion adjacent to the newly hydroxylated oxygen is extracted to the surface. (c-f) Repetition of these processes leads to the growth of $OH^-$ rows along the [111] direction. Terrace dissolution is essential for extracting buried $Mg^{2+}$ ions from the crystal lattice. This dissolution most likely involves additional elementary processes such as $Mg^{2+}$ dissolution and hydroxylation of surface oxygen atoms, but the details are omitted in this illustration for simplicity. Mg, O, and H atoms are colored gray, red, and white, respectively.

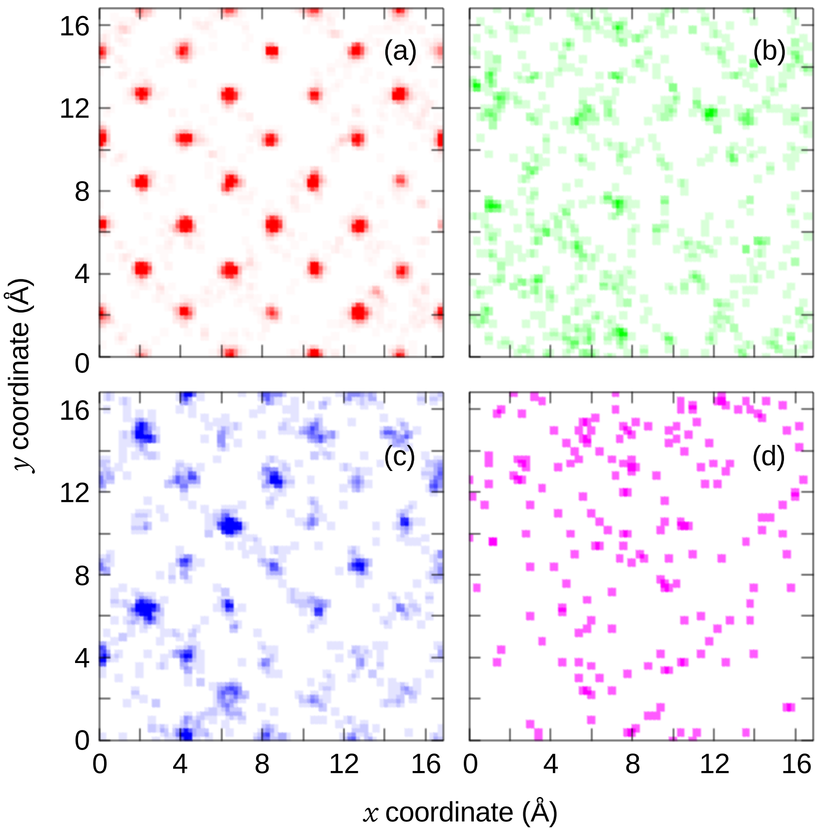


Figure S20: Normalized lateral distribution of dissolved $Mg^{2+}$ ions partitioned by their $z$ coordinate: (a) 1.0 Å to 3.0 Å, (b) 3.0 Å to 4.0 Å, (c) 4.0 Å to 5.0 Å, and (d) > 5.0 Å. The $Mg^{2+}$ ions are sampled from snapshots taken during PS-MD cycles 100 – 300, with respective sample size of (a) 34407, (b) 4713, (c) 4432, and (d) 435.

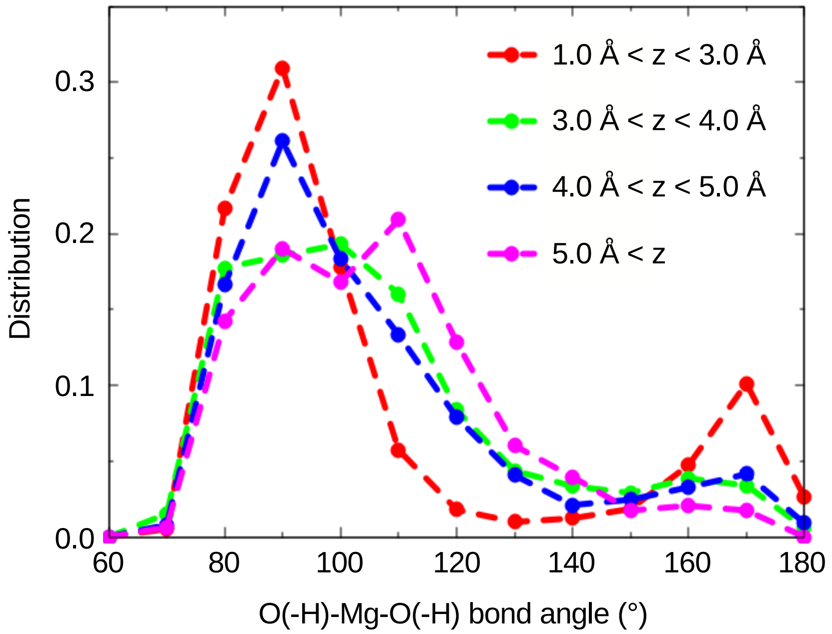


Figure S21: Bond angle distribution of O(-H)-Mg-O(-H) chains observed in the water layer, partitioned by the $Mg^{2+}$ ion's $z$ coordinate: 1.0 Å to 3.0 Å(red), 3.0 Å to 4.0 Å(green), 4.0 Å to 5.0 Å(blue), and > 5.0 Å(magenta).

## References


(S1) Inagaki, T.; Saito, S. Hybrid Monte Carlo method with potential scaling for sampling from the canonical multimodal distribution and imitating the relaxation process. *J. Chem. Phys.* **2022**, *156*, 104111.

(S2) Mark, A. E.; van Gunsteren, W. F.; Berendsen, H. J. C. Calculation of relative free energy via indirect pathways. *J. Chem. Phys.* **1991**, *94*, 3808–3816.

(S3) Tsujishita, H.; Moriguchi, I.; Hirono, S. Potential-scaled molecular dynamics and potential annealing: effective conformational search techniques for biomolecules. *J. Phys. Chem.* **1993**, *97*, 4416–4420.

(S4) Sinko, W.; Miao, Y.; de Oliveira, C. A. F.; McCammon, J. A. Population Based Reweighting of Scaled Molecular Dynamics. *J. Phys. Chem. B* **2013**, *117*, 12759–12768.

(S5) van Duin, A. C. T.; Dasgupta, S.; Lorant, F.; Goddard, W. A. ReaxFF: A Reactive Force Field for Hydrocarbons. *J. Phys. Chem. A* **2001**, *105*, 9396–9409.

(S6) Zhu, R.; Janetzko, F.; Zhang, Y.; van der Vaart, A.; Merz, K. M., Jr. Characterization of the active site of yeast RNA polymerase II by DFT and ReaxFF calculations. *Theor. Chem. Acc.* **2008**, *120*, 479–489.

(S7) Pathak, A. D.; Nedea, S.; van Duin, A. C. T.; Zondag, H.; Rindt, C.; Smeulders, D. Reactive force field development for magnesium chloride hydrates and its application for seasonal heat storage. *Phys. Chem. Chem. Phys.* **2016**, *18*, 15838–15847.

(S8) Thompson, A. P.; Aktulga, H. M.; Berger, R.; Bolintineanu, D. S.; Brown, W. M.; Crozier, P. S.; in 't Veld, P. J.; Kohlmeyer, A.; Moore, S. G.; Nguyen, T. D.; Shan, R.; Stevens, M. J.; Tranchida, J.; Trott, C.; Plimpton, S. J. LAMMPS - a flexible simulation tool for particle-based materials modeling at the atomic, meso, and continuum scales. *Comput. Phys. Commun.* **2022**, *271*, 108171.

(S9) Hazen, R. M. Effects of temperature and pressure on the cell dimension and X-ray temperature factors of periclase. *Am. Mineral.* **1976**, *61*, 266–271.

(S10) Zigan, F.; Rothbauer, R. Neutronenbeugungsmessungen am Bruci. *Neues Jahrb. Mineral., Monatsh* **1967**, *61*, 137–143.

(S11) Barin, I.; Platzki, G. *Thermochemical data of pure substances*, 3rd ed.; VCH: Weinheim; New York, 1995.

(S12) Jura, G.; Garland, C. W. The Experimental Determination of the Surface Tension of Magnesium Oxide. *J. Am. Chem. Soc.* **1952**, *74*, 6033–6034.

(S13) Logsdail, A. J.; Mora-Fonz, D.; Scanlon, D. O.; Catlow, C. R. A.; Sokol, A. A. Structural, energetic and electronic properties of (100) surfaces for alkaline earth metal oxides as calculated with hybrid density functional theory. *Surf. Sci.* **2015**, *642*, 58–65.

(S14) Zhang, W.; Li, X.; Shan, Z.; Wang, S.; Xiao, Y. Surface modification of magnesium hydroxide by wet process and effect on the thermal stability of silicone rubber. *Appl. Surf. Sci.* **2019**, *465*, 740–746.

(S15) Churakov, S. V.; Iannuzzi, M.; Parrinello, M. Ab Initio Study of Dehydroxylation − Carbonation Reaction on Brucite Surface. *J. Phys. Chem. B* **2004**, *108*, 11567–11574.

(S16) McCarthy, M. I.; Schenter, G. K.; Scamehorn, C. A.; Nicholas, J. B. Structure and Dynamics of the Water/MgO Interface. *J. Phys. Chem.* **1996**, *100*, 16989–16995.

(S17) Hu, X. L.; Klimeš, J.; Michaelides, A. Proton transfer in adsorbed water dimers. *Phys. Chem. Chem. Phys.* **2010**, *12*, 3953–3956.

(S18) Ončák, M.; Włodarczyk, R.; Sauer, J. Hydration Structures of MgO, CaO, and SrO (001) Surfaces. *J. Phys. Chem. C* **2016**, *120*, 24762–24769.

(S19) Ding, Z.; Goldsmith, Z. K.; Selloni, A. Pathways for Electron Transfer at MgO–Water Interfaces from Ab Initio Molecular Dynamics. *J. Am. Chem. Soc.* **2022**, *144*, 2002–2009.

(S20) Odelius, M. Mixed Molecular and Dissociative Water Adsorption on MgO[100]. *Phys. Rev. Lett.* **1999**, *82*, 3919–3922.

(S21) Feyereisen, M. W.; Feller, D.; Dixon, D. A. Hydrogen Bond Energy of the Water Dimer. *J. Phys. Chem.* **1996**, *100*, 2993–2997.

(S22) Hourahine, B.; Aradi, B.; Blum, V.; Bonafé, F.; Buccheri, A.; Camacho, C.; Cevallos, C.; Deshaye, M. Y.; Dumitrică, T.; Dominguez, A.; Ehlert, S.; Elstner, M.; van der Heide, T.; Hermann, J.; Irle, S.; Kranz, J. J.; Köhler, C.; Kowalczyk, T.; Kubař, T.; Lee, I. S.; Lutsker, V.; Maurer, R. J.; Min, S. K.; Mitchell, I.; Negre, C.; Niehaus, T. A.; Niklasson, A. M. N.; Page, A. J.; Pecchia, A.; Penazzi, G.; Persson, M. P.; Řezáč, J.; Sánchez, C. G.; Sternberg, M.; Stöhr, M.; Stuckenberg, F.; Tkatchenko, A.; Yu, V. W.-z.; Frauenheim, T. DFTB+, a software package for efficient approximate density functional theory based atomistic simulations. *J. Chem. Phys.* **2020**, *152*, 124101.

(S23) Gaus, M.; Cui, Q.; Elstner, M. DFTB3: Extension of the Self-Consistent-Charge Density-Functional Tight-Binding Method (SCC-DFTB). *J. Chem. Theory Comput.* **2011**, *7*, 931–948.

(S24) Gaus, M.; Lu, X.; Elstner, M.; Cui, Q. Parameterization of DFTB3/3OB for Sulfur and Phosphorus for Chemical and Biological Applications. *J. Chem. Theory Comput.* **2014**, *10*, 1518–1537.

(S25) Lu, X.; Gaus, M.; Elstner, M.; Cui, Q. Parametrization of DFTB3/3OB for Magnesium and Zinc for Chemical and Biological Applications. *J. Phys. Chem. B* **2015**, *119*, 1062–1082.

(S26) Grimme, S.; Antony, J.; Ehrlich, S.; Krieg, H. A consistent and accurate ab initio parametrization of density functional dispersion correction (DFT-D) for the 94 elements H-Pu. *J. Chem. Phys.* **2010**, *132*, 154104.

(S27) Grimme, S.; Hansen, A.; Brandenburg, J. G.; Bannwarth, C. Dispersion-Corrected Mean-Field Electronic Structure Methods. *Chem. Rev.* **2016**, *116*, 5105–5154.

(S28) DiStasio, J., Robert A.; Santra, B.; Li, Z.; Wu, X.; Car, R. The individual and collective effects of exact exchange and dispersion interactions on the ab initio structure of liquid water. *J. Chem. Phys.* **2014**, *141*, 084502.

(S29) Giannozzi, P.; Andreussi, O.; Brumme, T.; Bunau, O.; Nardelli, M. B.; Calandra, M.; Car, R.; Cavazzoni, C.; Ceresoli, D.; Cococcioni, M.; Colonna, N.; Carnimeo, I.; Corso, A. D.; de Gironcoli, S.; Delugas, P.; Jr, R. A. D.; Ferretti, A.; Floris, A.; Fratesi, G.; Fugallo, G.; Gebauer, R.; Gerstmann, U.; Giustino, F.; Gorni, T.; Jia, J.; Kawamura, M.; Ko, H.-Y.; Kokalj, A.; Küçükbenli, E.; Lazzeri, M.; Marsili, M.; Marzari, N.; Mauri, F.; Nguyen, N. L.; Nguyen, H.-V.; de-la Roza, A. O.; Paulatto, L.; Poncé, S.; Rocca, D.; Sabatini, R.; Santra, B.; Schlipf, M.; Seitsonen, A. P.; Smogunov, A.; Timrov, I.; Thonhauser, T.; Umari, P.; Vast, N.; Wu, X.; Baroni, S. Advanced capabilities for materials modelling with QUANTUM ESPRESSO. *J. Phys. Condens. Matter* **2017**, *29*, 465901.

(S30) Delle Site, L.; Alavi, A.; Lynden-Bell, R. M. The structure and spectroscopy of monolayers of water on MgO: An ab initio study. *J. Chem. Phys.* **2000**, *113*, 3344–3350.

(S31) Otani, M.; Sugino, O. First-principles calculations of charged surfaces and interfaces: A plane-wave nonrepeated slab approach. *Phys. Rev. B* **2006**, *73*, 115407.

(S32) Sasahara, A.; Murakami, T.; Tomitori, M. Hydration of MgO(100) Surface Promoted at $\langle 011 \rangle$ Steps. *J. Phys. Chem. C* **2015**, *119*, 8250–8257.

(S33) Ding, Z.; Selloni, A. Hydration structure of flat and stepped MgO surfaces. *J. Chem. Phys.* **2021**, *154*, 114708.

(S34) Ishida, T.; Ishimura, K. Chemical Heat Storage Mechanism in Alkaline Earth Metal Oxide: Ab Initio Modeling of the Initial Hydration Reaction on MgO(001) Surface. *J. Phys. Chem. C* **2024**, *128*, 7397–7407.

(S35) Luong, N. T.; Boily, J.-F. Water Film-Driven Brucite Nanosheet Growth and Stacking. *Langmuir* **2023**, *39*, 11090–11098.

(S36) Thomele, D.; Gheisi, A. R.; Niedermaier, M.; Elsässer, M. S.; Bernardi, J.; Grönbeck, H.; Diwald, O. Thin water films and particle morphology evolution in nanocrystalline MgO. *J. Am. Ceram. Soc.* **2018**, *101*, 4994–5003.

(S37) Maltseva, A.; Shkirskiy, V.; Lefèvre, G.; Volovitch, P. Effect of pH on $Mg(OH)_2$ film evolution on corroding Mg by in situ kinetic Raman mapping (KRM). *Corros. Sci.* **2019**, *153*, 272–282.

(S38) Bracco, J. N.; Camacho Meneses, G.; Colón, O.; Yuan, K.; Stubbs, J. E.; Eng, P. J.; Wanhala, A. K.; Einkauf, J. D.; Boebinger, M. G.; Stack, A. G.; Weber, J. Reaction Layer Formation on MgO in the Presence of Humidity. *ACS Appl. Mater. Interfaces* **2024**, *16*, 712–722.

(S39) Pettauer, M.; Baldermann, A.; Eder, S.; Dietzel, M. Hydration of MgO: Reaction Kinetics and pH Control on Brucite Crystal Morphology. *Cryst. Growth Des.* **2024**, *24*, 3085–3092.

(S40) Kuleci, H.; Schmidt, C.; Rybacki, E.; Petrishcheva, E.; Abart, R. Hydration of periclase at 350 °C to 620 °C and 200 MPa: experimental calibration of reaction rate. *Miner. Petrol.* **2016**, *110*, 1–10.

(S41) Liu, P.; Kendelewicz, T.; Brown, G. E.; Parks, G. A. Reaction of water with MgO(100) surfaces. Part I:: Synchrotron X-ray photoemission studies of low-defect surfaces. *Surf. Sci.* **1998**, *412-413*, 287–314.

(S42) Mejias, J. A.; Berry, A. J.; Refson, K.; Fraser, D. G. The kinetics and mechanism of MgO dissolution. *Chem. Phys. Lett.* **1999**, *314*, 558–563.

(S43) Xie, C.; Yan, D.; Li, H.; Du, S.; Chen, W.; Wang, Y.; Zou, Y.; Chen, R.; Wang, S. Defect Chemistry in Heterogeneous Catalysis: Recognition, Understanding, and Utilization. *ACS Catal.* **2020**, *10*, 11082–11098.

(S44) Zhang, Y.; Tao, L.; Xie, C.; Wang, D.; Zou, Y.; Chen, R.; Wang, Y.; Jia, C.; Wang, S. Defect Engineering on Electrode Materials for Rechargeable Batteries. *Adv. Mater.* **2020**, *32*, 1905923.

(S45) Frankel, G. S. Pitting Corrosion of Metals: A Review of the Critical Factors. *J. Electrochem. Soc.* **1998**, *145*, 2186.

(S46) Giordano, L.; Goniakowski, J.; Suzanne, J. Partial Dissociation of Water Molecules in the (3×2) Water Monolayer Deposited on the MgO (100) Surface. *Phys. Rev. Lett.* **1998**, *81*, 1271–1273.

(S47) Errington, J. R.; Debenedetti, P. G. Relationship between structural order and the anomalies of liquid water. *Nature* **2001**, *409*, 318–321.
